# Supplementary material for: Improved Exploration in Factored Average-Reward MDPs
Source: arXiv:2009.04575 source file (2021-03-11)
Supplement: Supplementary file 2 [file simulation_appendix.tex]

\section{\uppercase{Further Numerical Experiments}}
\label{app:additional_sim}

In this section we present results from several additional experiments with \AlgB. We first perform a longer experiment in the Coffee domain \cite{boutilier1994fmdps}. Since the original experiment in Figure~\ref{fig:coffee-regret} does not clearly show the asymptotic behavior of the algorithms, we increase the time horizon tenfold to $10^7$. However, in this case we are only able to present an average of $4$ independent experiments. The regret of the three algorithms is shown in Figure~\ref{fig:coffee-10M}. \AlgB{} clearly reaches the sublinear domain within $2\cdot 10^6$ time steps, while UCRL-Factored and UCRLB continue to accumulate regret. Note the logarithmic scale on the y-axis, and that \AlgB{} outperforms the other algorithms by more than an order of magnitude after $10^7$ steps. As in Figure~\ref{fig:coffee-regret}, we omit UCRL-Factored-L since it does not outperform UCRL-Factored.

\begin{figure}
	\centering
	\caption{Regret in Coffee with time horizon $10^7$.}
	\label{fig:coffee-10M}
\end{figure}

We also perform two experiments in the SysAdmin domain \cite{guestrin2003fmdps}. This domain consists of $N$ computer servers that are organized in a graph with a certain topology. Each server is represented by a binary variable that indicates whether or not it is working. At each time step, each server has a chance of failing which depends on its own status and the status of the servers connected to it. There are $N+1$ actions: $N$ actions for rebooting a server (after which it works with high probability) and an idle action. In previous work, researchers have performed experiments with two different topologies: a circular topology in which each server is connected to the next server in the circle, and a three-legged topology in which the servers are organized in a tree with three branches. In each topology, the status of each server depends on at most one other server.

Figures~\ref{fig:circle-regret} and \ref{fig:threeleg-regret} show the regret of the four algorithms in the SysAdmin domain for the two topologies, averaged over 48 independent runs. For each topology, $N=7$, i.e.~the circular topology has 7 servers arranged in a circle, and the three-legged topology has a root server and two servers on each of the three branches. Hence the size of the state and action space is $S=2^7=128$, $A=8$, and $|\cX|=1024$. Note again the logarithmic scale on the y-axis. As in the other domains, \AlgB{} clearly outperforms the other algorithms in terms of regret. Also, UCRL-Factored-L clearly outperforms UCRL-Factored, and UCRL-Factored clearly outperforms UCRLB. The latter is interesting to note since UCRLB has much tighter confidence sets than UCRL-Factored, who benefits from the fact that the transition scopes are small in this domain.

\begin{figure}
	\centering
	\caption{Regret in SysAdmin with the circular topology.}
	\label{fig:circle-regret}
\end{figure}

\begin{figure}
	\centering
	\caption{Regret in SysAdmin with the three-legged topology.}
	\label{fig:threeleg-regret}
\end{figure}
